# Supplementary material for: KitcheNette: Predicting and Recommending Food Ingredient Pairings using Siamese Neural Networks
Source: arXiv:1905.07261 source file (2019-05-16)
Supplement: Supplementary file 1 [file _999_appendix.tex]

According to their hypothesis, two different ingredients that share a high number of compounds have a better flavor when used together in culinary practice. While they introduced a novel method for evaluating food pairings, their method has some limitations. For example, FlavorDB built by \cite{garg2017flavordb} contains only a limited number of flavor compounds and natural ingredients and a considerable amount of time and effort is required to analyze the flavor compounds of each food ingredient in FlavorDB. Moreover, chemical compound similarity is not the only factor that is used to evaluate food pairings. Some well-known food pairings consist of two completely different food ingredients (e.g., red wine and beef) that have very few flavor compounds in common.

The following three pairings are known to be excellent pairings. Gin\&Aquavit is one of the cocktail pairings widely used in the Nordic region. The pairing of Wasabi\&Nori in is common in Japanese cuisine but may be less popular in Western cuisine. The pairing of Lime\&Nopales is one of the pairings used in Mexican Cuisine.

The three examples of \textif{unknown} pairings that our model found are known to be excellent pairings. Gin\&Aquavit is one of the cocktail pairings widely used in the Nordic region. The pairing of Wasabi\&Nori in is common in Japanese cuisine but may be less popular in Western cuisine. The pairing of Lime\&Nopales is one of the pairings used in Mexican Cuisine.

(e.g., gin\&tonic water, salt\&pepper, vanilla\&onion) and then predicts scores for unknown food combinations (e.g., gin\&aquavit, lime\&nopales, wasabi\&nori)

which is a model that finds optimal ingredient pairings and discovers new parngs

\begin{table}[t]
    \centering
    \scalebox{0.8}{
    \begin{tabular}{c|cccc}
    \toprule
     & Ingredient1 & Ingredient2 & \begin{tabular}[c]{@{}c@{}}Pairing\\ Evaluation\end{tabular} & \begin{tabular}[c]{@{}c@{}}Score\\ (-1$\sim$1)\end{tabular} \\\midrule
    \multirow{3}{*}{\begin{tabular}[c]{@{}c@{}}Well-Known\\ Pairings\\(5\%)\end{tabular}} & Gin & Tonic Water & Good & 0.54 \\
     & Salt & Pepper & Good & 0.25 \\
     & Vanilla & Onion & Bad & -0.58 \\\midrule
     \multirow{3}{*}{\begin{tabular}[c]{@{}c@{}}Unknown\\Pairings\\(95\%)\end{tabular}} & Gin & \begin{tabular}[c]{@{}c@{}}Aquavit\end{tabular} & \textbf{\Large{?}} & \textbf{\Large{?}} \\     
     & Wasabi & Nori & \textbf{\Large{?}} & \textbf{\Large{?}} \\
     & Lime & Nopales & \textbf{\Large{?}} & \textbf{\Large{?}} \\\bottomrule
    \end{tabular}
    }
\end{table}

\section{\LaTeX{} and Word Style Files}\label{stylefiles}

Due the complexity of food itself and their countless combination possibilities, Food pairing has long been a field of comprehensive arts allowed only to a few experts. In this work, we introduce KichenNette that predicts and ranks food ingredient pairings based on a large amount of human experiences on foods. The model trains more than 300k food pairing scores of food ingredients from 1M human-written recipes on Siamese deep neural networks architecture. Our model outperforms the traditional machine learning methods and additional features and a pairing specific architecture enhance its performance. For analysis, we demonstrate that the results of our food pairing are more plausible to that of existing food pairing. Also, our model can successfully predict traditional drink-food pairing and the scores of food ingredient combinations that had never been tried before.

The \LaTeX{} and Word style files are available on the IJCAI--19
website, \url{http://www.ijcai19.org}.
These style files implement the formatting instructions in this
document.

The \LaTeX{} files are {\tt ijcai19.sty} and {\tt ijcai19.tex}, and
the Bib\TeX{} files are {\tt named.bst} and {\tt ijcai19.bib}. The
\LaTeX{} style file is for version 2e of \LaTeX{}, and the Bib\TeX{}
style file is for version 0.99c of Bib\TeX{} ({\em not} version
0.98i). The {\tt ijcai19.sty} style differs from the {\tt
ijcai18.sty} file used for IJCAI--18.

The Microsoft Word style file consists of a single file, {\tt
ijcai19.doc}. This template differs from the one used for
IJCAI--18.

These Microsoft Word and \LaTeX{} files contain the source of the
present document and may serve as a formatting sample.  

Further information on using these styles for the preparation of
papers for IJCAI--19 can be obtained by contacting {\tt
pcchair@ijcai19.org}.

%Pie Graph
% Plant/Vegetable 0.2238579855095843
% Sauce/Powder/Dressing 0.17951282464913695
% Cereal/Crop/Bean 0.07717233494883466
% Dairy 0.07444398465390631
% Spice 0.07409189420453509
% Meat/Animal Product 0.0713004201238629
% Fruit 0.060709651626840236
% Bakery/Dessert/Snack 0.048840977156203315
% Beverage 0.03777888439229329
% Beverage Alcoholic 0.03115228963998401
% Nut/Seed 0.029906646934638827
% Essential Oil/Fat 0.02868064274041395
% Seafood 0.0203693442841412
% Dish/End Product 0.015563520062843235
% Fungus 0.011812564438864614
% ETC 0.011484320752996626
% Flower 0.003321713880920485
\begin{figure}[!t]
    \centering
    \scalebox{0.75}{
    \begin{tikzpicture}
     \pie [text=pin, rotate=360,radius=2.5,
     color={red!40,orange!40,yellow!40,green!40,cyan!40,blue!40,purple!40,red!40,orange!20,yellow!70,black!40}]
        {22/Plant\&Vegetable,
         18/Sauce\&Powder\&Dressing,
         8/Cereal\&Crop\&Bean,
         7/Dairy,
         7/Spice,
         7/Meat\&Animal Product,
         6/Fruit,
         5/Bakery\&Dessert\&Snack,
         4/Beverage,
         3/Beverage Alcoholic,
         13/Others}
    \end{tikzpicture}
    }
    \caption{Ingredient Category}
    \label{figure:dataset-category}
\end{figure}

\begin{figure}[ht]
\begin{tikzpicture}
\begin{axis}[
        ymin=0, ymax=150000,
      scaled y ticks = false,
      y tick label style={/pgf/number format/fixed,
      /pgf/number format/1000 sep = \thinspace % Optional if you want to replace comma as the 1000 separator 
      }]    
\addplot+[ybar interval,mark=no] plot coordinates {(-1,	0)
(-0.9,	0)
(-0.8,	0)
(-0.7,	0)
(-0.6,	0)
(-0.5,	3)
(-0.4,	45)
(-0.3,	323)
(-0.2,	3282)
(-0.1,	21910)
(0,	88242)
(0.1,	139529)
(0.2,	72565)
(0.3,	21929)
(0.4,	6252)
(0.5,	1758)
(0.6,	491)
(0.7,	97)
(0.8,	22)
(0.9,	3)
(1	,0)};
\end{axis}
\end{tikzpicture}
\caption{-1 to 1 score distribution with 0.1 interval}
\end{figure}

Since our aim is to discover novel ingredient pairs by exploiting large-scale data, we look into previous works whose objective is similar to ours. One of the dominant hypotheses regarding food pairing is that ingredients with similar flavor compounds have stronger tendency to form pairs in culinary practice. \cite{ahn2011flavor} follows this hypothesis and creates a large-scale flavor network that illustrates flavor compound based similarities between ingredients. \cite{simas2017food} extends this hypothesis by introducing 'food bridging'. Food bridging assumes that two different ingredients that barely share chemical similarities can be connected by a series of intermediate adjacent ingredients in a flavor network. Thus, ingredients that are two or more hops away can form a new pair by a chain of affinities or chemical similarities.

We believe Ahn's hypothesis on food pairing is one-sided since ingredients that do not share chemical similarities can also form pairs as well. Our motive is to apply our novel data-driven method to a large-scale corpus and derive food pairings that are not always necessarily similar in terms of flavor compound and molecular properties. Therefore, our hypothesis focuses on finding new ingredient pairs in a data-driven way that encompasses not only ingredient pairs with similar chemical properties but also pairs that show strong contrast. To this extent, our work attempts to broaden the underlying concept of food pairing and introduce a data-driven, deep learning based approach for discovering novel ingredient pairs. 

\begin{table*}[!t]
    \centering
    \scalebox{0.75}{
    \begin{tabular}{c|c|cc|llllllllll}
    \toprule
     & Model & Input Type & Dist Func & Loss & MSE & MAE & CORR & R2 & Loss & MSE & MAE & CORR & R2 \\\midrule
    \multirow{6}{*}{\begin{tabular}[c]{@{}l@{}}Baseline\\ Models\end{tabular}} & Cosine Similiarity & Im2Recipe & - & - & - & - & - & - & 0.1802 & 0.0325 & 0.1328 & 0.3952 & -1.6026 \\
     & SGD & Im2Recipe & - & 0.0993 & 0.0099 & 0.0762 & 0.4585 & 0.2102 & 0.0984 & 0.0097 & 0.0759 & 0.4730 & 0.2236 \\
     & Extra Tree & Im2Recipe & - & 0.0742 & 0.0055 & 0.0566 & 0.7664 & 0.5586 & 0.0738 & 0.0054 & 0.0563 & 0.7689 & 0.5637 \\
     & Gradient Boosting & Im2Recipe & - & 0.1073 & 0.0115 & 0.0815 & 0.3339 & 0.0773 & 0.1073 & 0.0115 & 0.0815 & 0.3351 & 0.0776 \\
     & Random Forest & Im2Recipe & - & 0.0802 & 0.0064 & 0.0612 & 0.7015 & 0.4846 & 0.0799 & 0.0064 & 0.0611 & 0.7042 & 0.4885 \\
     & Linear SVR & Im2Recipe & - & 0.0993 & 0.0099 & 0.0762 & 0.4588 & 0.2105 & 0.0984 & 0.0097 & 0.0759 & 0.4731 & 0.2238 \\\midrule
    \multirow{6}{*}{\begin{tabular}[c]{@{}l@{}}KitcheNet\\ Models\end{tabular}} & KitcheNet1 & Im2Recipe & CROSSCAT & 0.0492 & 0.0025 & 0.0371 & 0.8968 & 0.8025 & 0.0488 & 0.0024 & 0.0368 & 0.8980 & 0.8053 \\
     & KitcheNet2 & \begin{tabular}[c]{@{}l@{}}Im2Recipe\\ +Category\end{tabular} & COSINE & 0.1002 & 0.0104 & 0.0705 & 0.6311 & 0.1642 & 0.0993 & 0.0102 & 0.0702 & 0.6398 & 0.1812 \\
     & KitcheNet3 & \begin{tabular}[c]{@{}l@{}}Im2Recipe\\ +Category\end{tabular} & CONCAT & 0.0511 & 0.0027 & 0.0388 & 0.8885 & 0.7867 & 0.0506 & 0.0026 & 0.0384 & 0.8909 & 0.7916 \\
     & KitcheNet4 & \begin{tabular}[c]{@{}l@{}}Random\\ +Category\end{tabular} & CROSSCAT & 0.0610 & 0.0038 & 0.0454 & 0.8452 & 0.6965 & 0.0602 & 0.0037 & 0.0449 & 0.8487 & 0.7040 \\
     & KitcheNet5 & \begin{tabular}[c]{@{}l@{}}Glove\\ +Category\end{tabular} & CROSSCAT & 0.0533 & 0.0029 & 0.0403 & 0.8775 & 0.7689 & 0.0527 & 0.0028 & 0.0399 & 0.8798 & 0.7734 \\
     & KitcheNet6 & \begin{tabular}[c]{@{}l@{}}Im2Recipe\\ +Category\end{tabular} & CROSSCAT & 0.0482 & 0.0024 & 0.0363 & 0.9008 & 0.8100 & 0.0478 & 0.0023 & 0.0360 & 0.9021 & 0.8134 \\\bottomrule
    \end{tabular}
    }
\end{table*}

\begin{tikzpicture}
\begin{axis}[
    title={TopN Accuracy},
    xlabel={TopN},
    ylabel={Accuracy},
    xmin=-0.5, xmax=5.5,
    ymin=0, ymax=1,
    xtick={0.0, 1.0, 2.0, 3.0, 4.0, 5.0},
    xticklabels={10,20,50,100,500,1000},
    ytick={0,0.20,0.40,0.60,0.80,1.00},
    legend pos=north west,
    ymajorgrids=true,
    grid style=dashed,
]
 
\addplot[
    color=blue,
    mark=square,
    ]
    coordinates {
    (0,0.2)(1,0.35)(2,0.54)(3,0.47)(4,0.58)(5,0.615)
    };
\addplot[
    color=red,
    mark=square,
    ]
    coordinates {
    (0,0.2)(1,0.25)(2,0.2)(3,0.2)(4,0.37)(5,0.429)
    };
\addplot[
    color=orange,
    mark=square,
    ]
    coordinates {
    (0,0)(1,0.1)(2,0.14)(3,0.21)(4,0.316)(5,0.374)
    };
\addplot[
    color=yellow,
    mark=square,
    ]
    coordinates {
    (0,0)(1,0)(2,0.08)(3,0.09)(4,0.222)(5,0.274)
    };
\addplot[
    color=green,
    mark=square,
    ]
    coordinates {
    (0,0)(1,0)(2,0.08)(3,0.09)(4,0.222)(5,0.275)
    };
\addplot[
    color=purple,
    mark=square,
    ]
    coordinates {
    (0,0)(1,0)(2,0)(3,0)(4,0.08)(5,0.114)
    };
    \legend{KitcheNet,et,rf,svr,sgd,gb}
\end{axis}
\end{tikzpicture}
